# Supplementary material for: Improving Primate Sounds Classification using Binary Presorting for Deep Learning
Source: arXiv:2306.16054 source file (2023-06-28)
Supplement: Supplementary file 1 [file 9_appendix.tex]

\section*{\uppercase{Appendix}}

If any, the appendix should appear directly after the
references without numbering, and not on a new page. To do so please use the following command:
\textit{$\backslash$section*\{APPENDIX\}}
